# Supplementary material for: Robust Real-Time Multi-View Eye Tracking
Source: arXiv:1711.05444 source file (2018-01-03)
Supplement: Supplementary file 1 [file main_SI.pdf]

# Robust Real-Time Multi-View Eye Tracking

## SUPPLEMENTARY INFORMATION

Nuri Murat Arar, *Student Member, IEEE,* and Jean-Philippe Thiran, *Senior Member, IEEE*

TABLE SI: Head pose statistics (in °) of two subjects from the dataset. The head pose angles are estimated with respect to the bottom camera view separately on calibration and six individual test sessions relevant to head movements.

| | Session | Exp No | Yaw | | | | Pitch | | | | Roll | | | |
|---|---|---|---|---|---|---|---|---|---|---|---|---|---|---|
| | | | Min | Max | Std | Mean | Min | Max | Std | Mean | Min | Max | Std | Mean |
| **Subject #8** | **Calibration** | #2 | -13.3 | 2.6 | 4.7 | -4.8 | -13.6 | 4.9 | 5.3 | -3.6 | -6.2 | 0.1 | 1.7 | -3.2 |
| | **Test** | #2 | -11.3 | 6.2 | 4.6 | -2.6 | -16.5 | 3.8 | 5.1 | -5.3 | -6.7 | 0.1 | 1.5 | -2.7 |
| | | #3 | -20.9 | 31.2 | 11.3 | -1.5 | -21.3 | 6.7 | 5.6 | -3.4 | -20.1 | 13.5 | 5.7 | -3.9 |
| | | #4 | -21.9 | 10.5 | 9.1 | -3.4 | -15.9 | 7.2 | 5.6 | -1.8 | -12.8 | 0.7 | 3.4 | -5.3 |
| | | #5 | -15.8 | 10.2 | 6.2 | -3.6 | -5.7 | 5.6 | 2.9 | -0.2 | -9.4 | 0.2 | 2.1 | -4.6 |
| | | #6 | -12.9 | 13.2 | 6.3 | -2.4 | -16.9 | 8.4 | 4.9 | -2.3 | -11.9 | -2.6 | 2.2 | -8.5 |
| | | #7 | -15.2 | 9.9 | 5.3 | -3.5 | -8.2 | 6.4 | 2.9 | -0.4 | -3.7 | 4.5 | 1.8 | 0.5 |
| **Subject #18** | **Calibration** | #2 | -14.1 | 22.9 | 13.5 | 2.6 | -21.1 | 0.9 | 6.9 | -9.6 | -4.4 | 4.4 | 2.4 | -0.6 |
| | **Test** | #2 | -15.8 | 22.9 | 12.3 | 3.7 | -23.1 | -0.7 | 7.1 | -10.2 | -4.2 | 2.4 | 1.6 | -1.1 |
| | | #3 | -24.5 | 19.4 | 10.4 | -0.9 | -20.8 | 7.9 | 6.2 | -7.4 | -25.5 | 16.7 | 8.7 | -2.7 |
| | | #4 | -18.1 | 22.9 | 12.7 | 0.2 | -24.3 | -1.9 | 6.2 | -12.6 | -6.3 | 1.9 | 2.2 | -1.6 |
| | | #5 | -15.7 | 19.1 | 10.5 | 0.6 | -21.3 | -2.3 | 4.7 | -10.2 | -5.4 | 1.9 | 1.4 | -2 |
| | | #6 | -18.1 | 18.9 | 10.2 | 1.9 | -22.9 | 3.6 | 7 | -8.4 | -14.2 | -6.5 | 1.6 | -9.4 |
| | | #7 | -17.2 | 28.2 | 11.9 | 3.6 | -22.6 | 4.9 | 6.8 | -7.8 | 1.1 | 7.4 | 1.6 | 4.4 |

TABLE SII: Mean estimation accuracy errors (°) and gaze availabilities (%) achieved by different setup configurations.

| | **Configurations** | | **Exp 0** | | **Exp 1** | | **Exp 2** | | **Exp 3** | | **Exp 4** | | **Exp 5** | | **Exp 6** | | **Exp 7** | |
|---|---|---|---|---|---|---|---|---|---|---|---|---|---|---|---|---|---|---|
| | camera | eye | (°) | (%) | (°) | (%) | (°) | (%) | (°) | (%) | (°) | (%) | (°) | (%) | (°) | (%) | (°) | (%) |
| **single-camera** | right | left | 1.71 | 50.6 | 1.68 | 51.6 | 1.59 | 57.3 | 2.04 | 46.8 | 1.87 | 36.3 | 2.06 | 49.6 | 1.84 | 51.1 | 1.53 | 37.5 |
| | right | right | 1.5 | 60.4 | 1.86 | 68.1 | 1.52 | 69.6 | 2.16 | 58.6 | 2.27 | 41.7 | 2.26 | 63.2 | 1.83 | 66.7 | 1.55 | 65.1 |
| | right | both | 1.55 | 74.4 | 1.6 | 74.9 | 1.41 | 77.6 | 2 | 69.7 | 2.11 | 52 | 2.07 | 75.2 | 1.77 | 73.7 | 1.35 | 69.4 |
| | left | left | 1.64 | 62.1 | 2.02 | 68.9 | 1.54 | 65.8 | 2.07 | 57 | 2.1 | 47.4 | 2.18 | 53.1 | 1.88 | 47.6 | 1.68 | 70.4 |
| | left | right | 1.55 | 51.4 | 1.86 | 56.1 | 1.49 | 56.9 | 1.86 | 44.2 | 1.83 | 44.7 | 2.28 | 51.2 | 2.08 | 33.8 | 1.75 | 62.1 |
| | left | both | 1.5 | 73.1 | 1.8 | 78.3 | 1.36 | 79.4 | 1.88 | 68.3 | 1.79 | 61.8 | 2.07 | 71.9 | 1.77 | 58.7 | 1.51 | 83.2 |
| | bottom | left | 1.68 | 77 | 1.86 | 78.1 | 1.50 | 81.8 | 1.93 | 72.1 | 1.96 | 64.7 | 1.99 | 67.7 | 1.79 | 77.6 | 1.63 | 73.4 |
| | bottom | right | 1.65 | 74.6 | 1.86 | 79.5 | 1.54 | 79.2 | 1.90 | 68.3 | 2.05 | 64.8 | 2.32 | 67.4 | 1.76 | 75.5 | 1.58 | 75.1 |
| | bottom | both | 1.46 | 91.2 | 1.51 | 94.6 | 1.30 | 93.6 | 1.67 | 87 | 1.73 | 82.4 | 1.81 | 83.9 | 1.33 | 92.5 | 1.32 | 90.8 |
| **multi-view** | overall | | 1.07 | 96.2 | 1.22 | 98.4 | 0.99 | 97.2 | 1.45 | 92.2 | 1.52 | 92.4 | 1.60 | 93.7 | 1.10 | 95.2 | 1.12 | 95.5 |
| | w/ perfect vis. | | 0.86 | 98 | 1.02 | 98.5 | 0.77 | 98.8 | 1.20 | 94.8 | 1.21 | 94.9 | 1.18 | 98.8 | 0.79 | 98.8 | 0.81 | 98.9 |
| | w/ contacts | | 0.83 | 96.8 | 1.05 | 99.7 | 0.76 | 98.9 | 1.23 | 92.5 | 1.41 | 97.5 | 1.17 | 99.1 | 0.88 | 99 | 1.02 | 98.5 |
| | w/o glasses | | 0.98 | 97 | 1.11 | 99.1 | 0.89 | 98.6 | 1.38 | 94.2 | 1.40 | 96.5 | 1.44 | 96.8 | 0.92 | 98.9 | 1.01 | 98.3 |
| | w/ glasses | | 1.39 | 93.4 | 1.63 | 95.6 | 1.38 | 91.9 | 1.68 | 84.4 | 1.95 | 76.8 | 2.19 | 82 | 1.77 | 81.4 | 1.51 | 85 |
| | dark-eyed | | 0.92 | 96.7 | 1.16 | 97.8 | 0.86 | 98.2 | 1.29 | 93.8 | 1.42 | 93.5 | 1.46 | 96.4 | 1.05 | 95.9 | 1.03 | 97 |
| | light-eyed | | 1.33 | 95.4 | 1.33 | 99.3 | 1.22 | 95.7 | 1.70 | 89.5 | 1.68 | 90.5 | 1.85 | 89.1 | 1.18 | 94 | 1.26 | 93 |

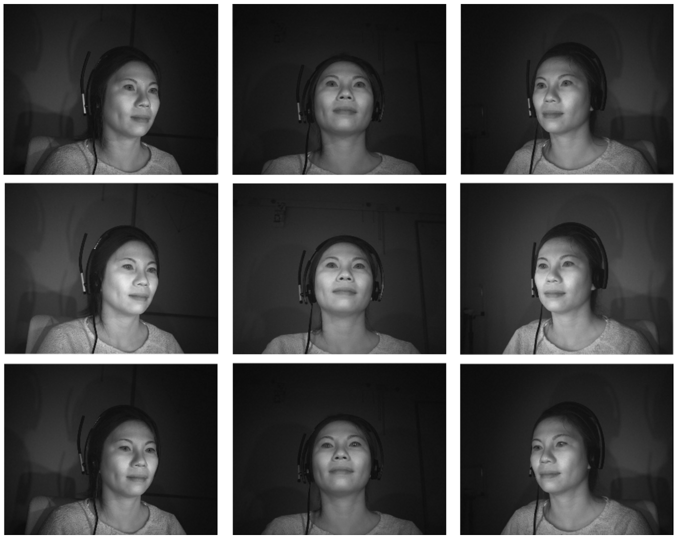

(a) Illumination variations, i.e., experiments #2, #0, #1.

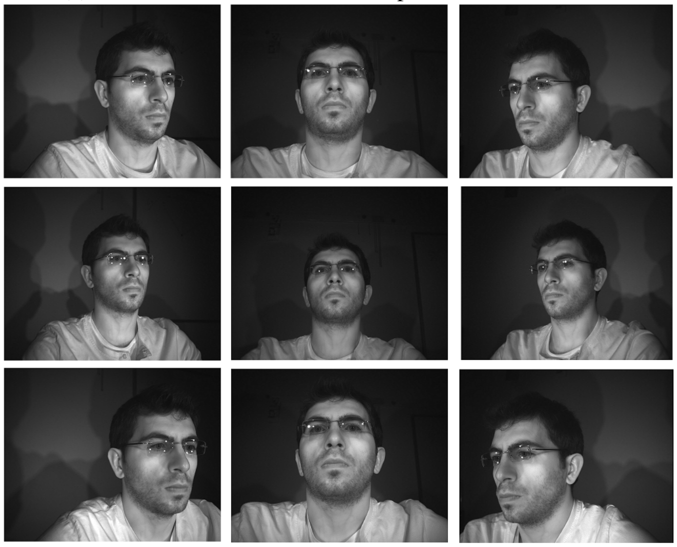

(b) Depth movements, i.e., experiments #2, #5, #4.

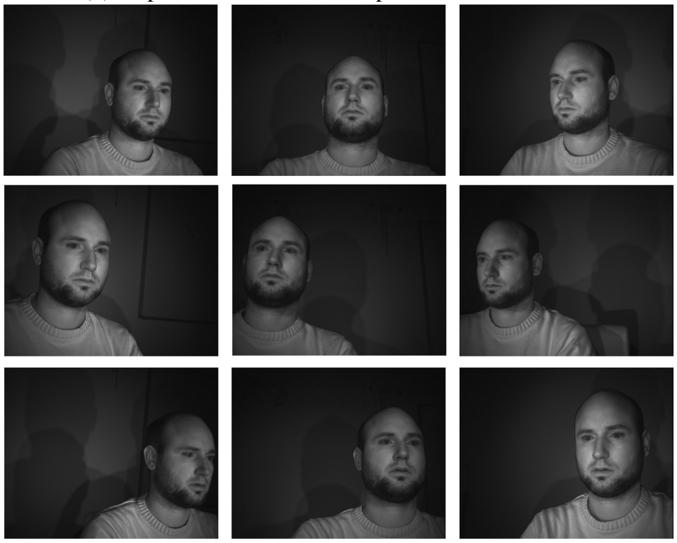

(c) Horizontal movements, i.e., experiments #2, #6, #7.

Fig. S1: Sample images from the collected dataset: (left column) right camera view, (middle column) bottom camera view, and (right column) left camera view.
